# Supplementary material for: Extreme Multi-label Completion for Semantic Document Labelling with Taxonomy-Aware Parallel Learning
Source: arXiv:2412.13809 source file (2024-12-18)
Supplement: Supplementary file 1 [file appendix.tex]

\section{Additional Experimental Results}

\subsection{Distribution over tasks}
In this section we report the  results on our XMLCo experiments for each task, presented as a distribution of the Precision and NDGC metrics values for MAG-CS, PubMed and EURLex datasets, respectively).

\ja{Quickly discuss the results here once ready.}

\begin{figure*}[!t]
	\centering
  \begin{subfigure}[t]{0.48\textwidth}
        \centering
        \includegraphics[width=0.95\textwidth]{figures/precision@_1_MAG-CS.png}
        \caption{MAG-CS - Precision@1}
    \end{subfigure}
    \begin{subfigure}[t]{0.48\textwidth}
        \centering
        \includegraphics[width=0.95\textwidth]{figures/ndcg@_2_MAG-CS.png}
        \caption{MAG-CS - NDCG@2}
    \end{subfigure}
     \begin{subfigure}[t]{0.48\textwidth}
        \centering
        \includegraphics[width=0.95\textwidth]{figures/precision@_2_MAG-CS.png}
        \caption{MAG-CS - Precision@2}
    \end{subfigure}
    \begin{subfigure}[t]{0.48\textwidth}
        \centering
        \includegraphics[width=0.95\textwidth]{figures/ndcg@_3_MAG-CS.png}
        \caption{MAG-CS - NDCG@3}
    \end{subfigure}
     \begin{subfigure}[t]{0.48\textwidth}
        \centering
        \includegraphics[width=0.95\textwidth]{figures/precision@_3_MAG-CS.png}
        \caption{MAG-CS - Precision@3}
    \end{subfigure}
    \begin{subfigure}[t]{0.48\textwidth}
        \centering
        \includegraphics[width=0.95\textwidth]{figures/ndcg@_4_MAG-CS.png}
        \caption{MAG-CS - NDCG@4}
    \end{subfigure}
	
	% \vspace{-0.2in}
	\caption{\ja{PLACEHOLDER FIGURES} Comparison of the distribution of performance of \algoName and other competing methods on the different TATs for the XMLCo experiment on the MAG-CS Dataset.}
	\label{fig:class_metrics_eurlex}
	%\vspace{0.05in}
\end{figure*}

\begin{figure*}[!t]
	\centering
  \begin{subfigure}[t]{0.48\textwidth}
        \centering
        \includegraphics[width=0.95\textwidth]{figures/precision@_1_EURLex.png}
        \caption{EURLex - Precision@1}
    \end{subfigure}
    \begin{subfigure}[t]{0.48\textwidth}
        \centering
        \includegraphics[width=0.95\textwidth]{figures/ndcg@_2_EURLex.png}
        \caption{EURLex - NDCG@2}
    \end{subfigure}
     \begin{subfigure}[t]{0.48\textwidth}
        \centering
        \includegraphics[width=0.95\textwidth]{figures/precision@_2_EURLex.png}
        \caption{EURLex - Precision@2}
    \end{subfigure}
    \begin{subfigure}[t]{0.48\textwidth}
        \centering
        \includegraphics[width=0.95\textwidth]{figures/ndcg@_3_EURLex.png}
        \caption{EURLex - NDCG@3}
    \end{subfigure}
     \begin{subfigure}[t]{0.48\textwidth}
        \centering
        \includegraphics[width=0.95\textwidth]{figures/precision@_3_EURLex.png}
        \caption{EURLex - Precision@3}
    \end{subfigure}
    \begin{subfigure}[t]{0.48\textwidth}
        \centering
        \includegraphics[width=0.95\textwidth]{figures/ndcg@_4_EURLex.png}
        \caption{EURLex - NDCG@4}
    \end{subfigure}

	% \vspace{-0.2in}
	\caption{\ja{NOT FINAL FIGURES} Comparison of the distribution of performance of \algoName and other competing methods on the different TATs for the XMLCo experiment on the EURLex Dataset.}
	\label{fig:class_metrics_eurlex}
	%\vspace{0.05in}
\end{figure*}
